# Supplementary material for: Off-Policy Imitation Learning from Observations
Source: arXiv:2102.13185 source file (2021-02-25)
Supplement: Supplementary file 1 [file proof_backup.tex]

\section{Appendix}  
% Based on the assumption, we have the following lemma:
We refer the following lemma from \cite{yang2019imitation} for a coherent presentation:
{\lemma \label{theorem:kl}
%\textbf{Lemma:}
    \begin{align*}
        \KL(\mupi(s,a,s') || \mut(s,a,s')) = \KL(\mupi(s,a) || \mut(s,a)) 
    \end{align*}
}
\begin{proof}
\begin{align*}
    \KL(\mupi(s,a,s') || \mut(s,a,s')) 
    &= \int_{\cS \times \cA \times \cS} \mupi(s,a, s') \log \frac{\mupi(s,a) \cdot \cP(s'|s,a)}{\mut(s,a) \cdot \cP(s'|s,a)} ds da \\
    &=\int_{\cS \times \cA \times \cS} \mupi(s,a, s') \log \frac{\mupi(s,a)}{\mut(s,a)} ds da ds \\
    &= \KL(\mupi(s,a) || \mut(s,a)) 
\end{align*}
\end{proof}


% \subsection{}  \label{appendix:gap-KL}
% %\eq{\ref{eq:gap-KL}}: 
% $$\KL(\mupi(s,a) || \mut(s,a)) = \KL(\mupi(s)||\mut(s)) + \cD_\KL(\pi(a|s)||\pi_E(a|s)).$$

% \begin{proof}
% \begin{align*}
%    \KL(\mupi(s,a) || \mut(s,a)) &= \int_{\cS \times \cA} \mupi(s,a) \log \frac{\mupi(s,a)}{\mut(s,a)} ds da \\
%    &= \int_{\cS \times \cA} \mupi(s,a) \log \frac{\mupi(s) \pi(a|s)}{\mut(s) \pi_E(a|s)} ds da \\ 
%    &= \int_{\cS \times \cA} \mupi(s,a) \big (\log \frac{\mupi(s) }{\mut(s) } + \log \frac{\pi(a|s)}{ \pi_E(a|s)} \big ) ds da \\ 
%    &= \int_{\cS \times \cA} \mupi(s) \log \frac{\mupi(s) }{\mut(s) } ds + \int_{\cS \times \cA} \mupi(s,a) \log \frac{\pi(a|s)}{ \pi_E(a|s)} \big ) ds da \\
%    &= \KL(\mupi(s)||\mut(s)) + \cD_\KL(\pi(a|s)||\pi_E(a|s))
% \end{align*}
% \end{proof}

% A similar equation has been derived by \cite{yang2019imitation}:
% $$\KL(\mupi(s,a) || \mut(s,a)) = \KL(\mupi(s,s')||\mut(s,s')) + \cD_\KL(\mupi(a|s,s')||\pi_E(a|s,s')).$$
% \begin{proof}
% \begin{align*}
%    \KL(\mupi(s,a) || \mut(s,a)) &= \int_{\cS \times \cA \times \cS} \mupi(s,a, s') \log \frac{\mupi(s,a, s')}{\mut(s,a, s')} ds da ds' \\
%    &= \int_{\cS \times \cA \times \cS} \mupi(s,a, s') \log \frac{\mupi(s,s') \mupi(a|s,s')}{\mut(s,s') \mut(a|s,s')} ds da ds'\\ 
%    &= \int_{\cS \times \cA  \times \cS} \mupi(s,a,s') \big (\log \frac{\mupi(s,s') }{\mut(s,s') } + \log \frac{\mupi(a|s,s')}{ \mut(a|s,s')} \big ) ds da ds'\\ 
%    &= \int_{\cS \times \cS} \mupi(s,s') \log \frac{\mupi(s,s') }{\mut(s,s') } ds ds' + \int_{\cS \times \cA \times \cS} \mupi(s,a, s') \log \frac{\mupi(a|s,s')}{ \mut(a|s,s')} \big ) ds da ds'\\
%    &= \KL(\mupi(s,s')||\mut(s,s')) + \cD_\KL(\mupi(a|s,s')||\pi_E(a|s,s'))
% \end{align*}
% \end{proof}

\subsection{} \label{appendix:eq-main}
%\eq{\ref{eq:main}}:
\begin{align*}
    \KL(\mupi(s,s') || \mut(s,s')) \leq \cE_{(s,s')\sim \mupi(s,s')} [\log \frac{\muR(s,s')} {\mut(s,s')}] + \KL[\mupi(s,a) || \muR(s,a)]. 
\end{align*}

\begin{proof}
    \begin{align*}
        \KL(\mupi(s,s') || \mut(s,s'))  &= \int_{\cS \times \cA} \mupi(s,s') \log \frac{\mupi(s,s')}{\mut(s,s')} ds da \\
        &= \int_{\cS \times \cA} \mupi(s,s') \log \Big (\frac{\muR(s,s')} {\mut(s,s')} \cdot \frac{\mupi(s,s')} {\muR(s,s')} \Big )ds da \\
        &= \int_{\cS \times \cA} \mupi(s,s') \log \frac{\muR(s,s')} {\mut(s,s')} ds da + \int_{\cS \times \cA} \mupi(s,s') \log  \frac{\mupi(s,s')} {\muR(s,s')} ds da \\
        &= \cE_{(s,s')\sim \mupi(s,s')} [\log \frac{\muR(s,s')} {\mut(s,s')}] + \KL[\mupi(s,s') || \muR(s,s')]  
    \end{align*}


\end{proof}  

\subsection{} \label{Appendix:lfo-upperbound}
{\assumption{} \label{assume:bounded}
We assume that the density ratios $ \frac{\mupi(s,a)}{\mut(s,a)}$ and $\frac{\mupi(s,a)}{\muE(s,a)}$ are bounded by some finite constant: $$ \exists R_{\text{max}} > 0, \st ~\frac{\mupi(s,a)}{\mut(s,a)} \leq R_{\text{max}}, \frac{\mupi(s,a)}{\muR(s,a)} \leq R_{\text{max}}.$$
}

Based on the above assumption, we have Lemma \ref{lemma:lfo-upperbound}:
\begin{align*}
  \cE_{(s,a)\sim \mupi(s,a)} [\log \frac{\muR(s,a)} {\mut(s,a)}] \leq \cE_{(s, s')\sim \mupi(s, s')}[\log \frac {\muR(s,s')} {\mut(s,s')} ] + C
\end{align*}
%\textbf{Proof of Lemma \ref{lemma:lfo-upperbound}:}

\begin{proof}
\begin{align*}
    &\cE_{(s,a)\sim \mupi(s,a)} [\log \frac{\muR(s,a)} {\mut(s,a)}] = \int_{\cS \times \cA \times \cS } \mupi(s, a) \log \frac {\muR(s,a)} {\mut(s,a)}  ds da \\
    &= \underbrace{\int_{\cS \times \cA \times \cS } \mupi(s, a, s') \log \frac {\muR(s,a, s')} {\mut(s,a, s')}  ds da ds'}_{\text{Lemma \ref{theorem:kl}}}  \\
    &= \int_{\cS \times \cA \times \cS } \mupi(s, a, s') \log \Big ( \frac {\muR(s, s')} {\mut(s,s')} \cdot \frac{\muR(a|s,s')} {\mut(a|s,s')} \Big ) ds da ds' \\
    &= \int_{\cS \times \cA \times \cS } \mupi(s, a, s') \log  \frac {\muR(s, s')} {\mut(s,s')} ds da ds' + \int_{\cS \times \cA \times \cS } \mupi(s, a, s') \log \frac{\muR(a|s,s')} {\mut(a|s,s')}  ds da ds' \\
    %%%%%%
    &= \int_{\cS \times \cA \times \cS } \mupi(s, a, s') \log  \frac {\muR(s, s')} {\mut(s,s')} ds da ds' + \int_{\cS \times \cA \times \cS } \mupi(s, a, s') \Big ( \log \frac{\muR(a|s,s')} {\mupi(a|s,s')}  + \log \frac{\mupi(a|s,s')}{\mut(a|s,s')} \Big) ds da ds' \\
    %%%%
    &= \cE_{(s, s')\sim \mupi(s, s')}[\log \frac {\muR(s,s')} {\mut(s,s')} ]  - \cD_\KL[\mupi(a|s,s') || \muR(a|s,s')] +  \cD_\KL[\mupi(a|s,s') || \mut(a|s,s')\\
    &\leq \cE_{(s, s')\sim \mupi(s, s')}[\log \frac {\muR(s,s')} {\mut(s,s')} ] +  \cD_\KL[\mupi(a|s,s') || \mut(a|s,s')\\
    &= \cE_{(s, s')\sim \mupi(s, s')}[\log \frac {\muR(s,s')} {\mut(s,s')} ] + \underbrace{\KL[\pi(a|s)||\pi_E(a|s)] - \cD_\KL[\mupi(s'|s) || \mut(s'|s)}_{\text{Lemma \ref{lemma:bc-lowerbound-reverse}}}\\
    &\leq \cE_{(s, s')\sim \mupi(s, s')}[\log \frac {\muR(s,s')} {\mut(s,s')} ] +  \KL[\pi(a|s)||\pi_E(a|s)]  \\
    %&\leq \cE_{(s, s')\sim \mupi(s,   s')}[\log \frac {\muR(s,s')} {\mut(s,s')} ]   +  \sup_{\pi } \cD_\KL[\mupi(a|s,s') || \mut(a|s,s')] \\
    &= \cE_{(s, s')\sim \mupi(s,   s')}[\log \frac {\muR(s,s')} {\mut(s,s')} ]   +  C\\
    %%%%%%% 
    \end{align*}
    where $C = \sup_{\pi} \cD_\KL[\mupi(a|s,s') || \mut(a|s,s')]$ is bounded given assumption \ref{assume:bounded}.
\end{proof}

Noted that the last term,  $\sup_{\pi } \cD_\KL[\mupi(a|s,s') || \mut(a|s,s')] $ requires knowlge of expert action labels and therefore cannot be estimated, unless in a deterministic and injective MDP.
  
%  Here, we slightly abuse $\pi_R(a|s)$ to denote:  
%      $$\pi_R(a|s) = \int_{\cS} \muR(a|s,s') ds' = \int_{\cS} \frac{\muR(s,a,s')}{\muR(s,s')} ds' = \frac{\muR(s,a)}{\muR(s)} \leq 1.$$

\textbf{ Remark \ref{lemma:divergence}:} \textit{For distributions $P$ and $Q$, and a convex $f$-function with $f(x)=\frac{1}{2} x^2$, we have
\begin{align*}
    \cD_\KL[P||Q] \leq \cD_f[P||Q]. 
\end{align*} 
\vskip -0.1in
}
\begin{proof}

Given two distributions $P$ and $Q$, define their density ratio as $w_{p|q}= \frac{p(x)}{q(x)} \geq 0$. 
%
If we consdier a function $g(w)= w \log(w) - \frac{1}{2} w^2$, $g(w)$ is constantly decreasing when $w \in (0, \infty)$, as $\frac{\partial g} {\partial w}=\log w+ 1 - w \leq 0 ~\forall w \geq 0$.

Since KL-Divergence is a special case of $f$-divergence with $f_{\KL}(x)=x \log x$, it is sufficient to show that:
\begin{align*}
    \cD_{\KL}[P||Q] - \cD_f[P||Q]  &= \int_\cX q(x)  \Big (w_{p/q} \log(w_{p/q}) - \frac{1}{2} (w_{p/q})^2 \Big ) dx \\
    &\leq \int_\cX q(x) \sup_{w \in (0,+\infty)} (w \log(w) - \frac{1}{2} w^2 ) dx \\
    &= \int_\cX q(x) \lim_{w \to 0^+} (w \log(w) - \frac{1}{2} w^2 ) dx \\
    &= 0.
\end{align*}
\end{proof}

\subsection{Inverse Model Constraints} \label{appendix:inverse-proof} 
%  

{\assumption \label{assume:mdp}
    We assume the MDP is deterministic: 
    %$$\cP(s'|s,a)=\delta(s' - g(s,a)),$$ 
    %$\delta$ a Dirac delta function,  
    $$\exists g:\cS \times \cA \to \cS \text{ a deterministic function, }  \st ~\cP(s'|s,a) = 0~\forall s' \neq g(s,a).$$
}  

{\assumption \label{assume:support}
We assume that the support of expert transition distribution $\mut(s,s')$ is covered by $\muR(s,s')$: 
    $$\mut(s,s') > 0 \Longrightarrow \muR(s,s') > 0.$$
}


{\remark \label{remark:optimal-inverse}
Given arbitrary policy $\pi$, and a policy $\bpi$, $\st ~\bpi(a|s) \propto \muR(a|s,s') ~\forall (s,s') \sim \mut(s,s')$,
$$ \cD_\KL[\mut(s'|s)||\mupi(s'|s)] \geq \cD_\KL[\mut(s'|s)||\mu^\bpi(s'|s)].$$
}
We provide proof in a tabular case:
\begin{proof}
    \begin{align*}
        &\cD_\KL[\mut(s'|s)||\mu^\bpi(s'|s)] \\
        &= \cE_{(s,s') \sim \mut(s,s') } \big[  \log \frac{\mut(s'|s)}{\mu^\bpi(s'|s)} \big] \\
        &= \underbrace{ \cE_{(s,s')\sim \mut(s,s') } [\log \mut(s'|s)] }_{\text{fixed } \wrt \pi}- \cE_{(s,s')\sim \mut(s,s') }\log \mu^\bpi(s'|s) \\
        &= H(\mut(s'|s))  - \cE_{(s,s') \sim \mut(s,s')}\big[ \log \cE_{a\sim\bpi(\cdot|s)} [\cP(s'|s,a)] \big]\\ 
        &= H(\mut(s'|s))  - \underbrace{\cE_{(s,s') \sim \mut(s,s')}\big[ \log \cE_{a\sim\bpi(\cdot|s)} [1] \big]}_{\text{Assumption \ref{assume:mdp}}}\\ 
        &= H(\mut(s'|s)). \\ 
    \end{align*}
    Noted that given Assumption \ref{assume:support}, $\forall (s,s') \sim \mut(s,s'),$  $\muR(s,s')  > 0$. Combine with Assumption \ref{assume:mdp}: $$\forall (s,s') \sim \mut(s,s'), \bpi(a|s) > 0 \Longrightarrow \muR(a|s,s') > 0 \Longrightarrow \cP(a|s,s') = 1.$$

    At the meantime:
    \begin{align*}
        &\cD_\KL[\mut(s'|s)||\mupi(s'|s)] \\
        &= H(\mut(s'|s))  - \cE_{(s,s') \sim \mut(s,s')}\big[ \log \cE_{a\sim\pi(\cdot|s)} [\cP(s'|s,a)] \big]\\ 
        &\leq H(\mut(s'|s))  - \cE_{(s,s') \sim \mut(s,s')}\big[ \log \cE_{a\sim\pi(\cdot|s)} [1] \big]\\ 
        &= H(\mut(s'|s)).\\ 
    \end{align*}

    Based on the above we conclude:
    $$\cD_\KL[\mut(s'|s)||\mu^\bpi(s'|s)] \leq \cD_\KL[\mut(s'|s)||\mupi(s'|s)].$$
\end{proof}
% {\remark \label{remark:optimal-inverse}
% For arbitrary policy $\pi$, and for any off-policy distribution $\muR$ which satisfies Assumption \ref{assume:support}, we have the following property:
% \begin{small}
%    \begin{align*}
%     %\cE_{(s,s') \sim \mut(s,s')}\Big[ \log \Big( \pi(a|s) \cP(s'|s,a) \Big) \Big]  \leq \cE_{(s,s') \sim \mut(s,s')}\Big[ \log \Big(\muR(a|s,s') \cP(s'|s,a) \Big)\Big]
%     \cE_{(s,s') \sim \mut(s,s')} \cE_{a \sim \pi(\cdot|s)}[\cP(s'|s,a)] \leq  \cE_{a \sim \muR(\cdot|s,s')}[\cP(s'|s,a)].
%     %= \int_{\cA \times \cS \times \cS} \mut(s,s') \log \pi(a|s) \cP(s'|s,a) da ds' ds  \leq \int_{\cA \times \cS \times \cS } \muR(a|s,s') \cP(s'|s,a) da ds' ds.
%    \end{align*}
% \end{small}
% }

% We provide proof in a tabular setting.
% \begin{proof}
% Based on Assumption \ref{assume:mdp}, for arbitrary $\muR$, we have:
% \begin{align}
%     %\forall &(s,s') \sim \mut(s,s'), \nonumber\\
%     \muR(a|s,s') > 0 \Longrightarrow \muR(s,a)\cP(s'|s,a) > 0 \Longrightarrow  \cP(s'|s,a) = 1, \label{backward}
% \end{align}

% which leads to the following:
% \begin{align*}
%    % &\cE_{s' \sim \mut(s'|s)}\Big[   \muR(a|s,s') \cP(s'|s,a)  \Big] \\
%   %& \int_{\cA} \muR(a|s,s') \cP(s'|s,a) da  \\
%   %= & \int_{a \sim \cA, g(s,a)=s'} \muR(a|s,s') \delta(0) da + \int_{a \sim \cA, g(s,a) \neq s'} \muR(a|s,s') \delta(s' - g(s,a)) da \\
% %   = & \int_{\cA } \underbrace{\muR(a|s,s')\delta(0) da }_\text{\eq{\ref{backward}}} \\
% %   = & \delta(0)
% \forall (s,s') \sim \muR(s,s'), \cE_{a \sim \muR(\cdot|s,s')} [\cP(s'|s,a)] = \cE_{a \sim \muR(\cdot|s,s')}[1] = 1.
% \end{align*}
% %
% On the other hand:
% \begin{align*}
%     % \forall (s,s') \sim \mut(s,s'), & \int_{a \sim \cA} \pi(a|s) \cP(s'|s,a) da \\
%     % = & \int_{a \sim \cA} \pi(a|s) \delta(s' - g(s,a)) da \\
%     % \leq & \int_{a \sim \cA} \pi(a|s) \delta(0) da\\
%     % = & \delta(0) 
%     \forall (s,s') \sim \muR(s,s'), \cE_{a \sim \pi(\cdot|s)} [\cP(s'|s,a)] \leq \cE_{a \sim \muR(\cdot|s,s')}[1] = 1.
% \end{align*}
% Combining above leads to:
% $$\forall (s,s') \sim \muR(s,s'), \cE_{a \sim \pi(\cdot|s)}[\cP(s'|s,a)] \leq  \cE_{a \sim \muR(\cdot|s,s')}[\cP(s'|s,a)]. $$
% Based on Assumption \ref{assume:support}:
% $$\cE_{(s,s') \sim \mut(s,s')} \Big[\cE_{a \sim \pi(\cdot|s)}[\cP(s'|s,a)] \Big]\leq  \cE_{a \sim \muR(\cdot|s,s')}[\cP(s'|s,a)]$$ 
% \end{proof}

% \textbf{Remark \ref{remark:inverse-constraint}:}
% $$\pi(\cdot|s) \propto \PI^*(\cdot|s,s'), \forall (s, s') \sim \mut(s,s') \Longrightarrow \pi = \arg \min_\pi \cD_\KL[\mut(s'|s) || \mupi(s'|s)].$$
% \begin{proof}
% Assume that we have learn an optimal inveres model with $\PI^*=\muR(a|s,s)$, it naturally holds that:
% \begin{align} \label{eq:inverse}
%     \forall (s,s') \sim \mut(s,s'), \underbrace{\int_{\cA} \pi(a|s) \cP(s'|s,a) da  \leq \int_{\cA} \PI^*(a|s,s') \cP(s'|s,a)}_\text{Lemma \ref{remark:optimal-inverse}} da. 
% \end{align} 

% Let us define the \textit{forward state-transition distribution} induced by $\pi$ as $\mupi(s’|s)$: $$\mupi(s’|s)= \int_\cA \pi(a|s) \cP(s'|s,a) da,$$ and the same for $\mut(s’|s)$.
% %
% Now consider the \textit{conditional} $\KL$-divergence between $\mut(s'|s)$ and $\mupi(s'|s)$:
% \begin{align*}
%     %\arg \min_\pi
%     &- \cD_\KL[\mut(s'|s) || \mupi(s'|s)] := - \int_{\cS \times   \cS} \mut(s) \mut(s'|s) \log \frac{\mut(s’|s) }{\mupi(s’|s) } ds' ds \\
%     &= - \int_{\cS \times   \cS} \mut(s) \mut(s'|s) \log  \mut(s’|s) ds ds' + \int_{\cS \times   \cS} \mut(s) \mut(s'|s) \log  \mupi(s’|s) ds' ds  \\
%     &= \underbrace{H(\mut(s'|s))}_{\text{not optimizable~} \wrt \pi} + \int_{\cS \times   \cS} \mut(s) \mut(s'|s)  \log  \mupi(s’|s) ds' ds \\
%     &= H(\mut(s'|s))   +  \lkxcom{\max_{\pi}} \int_{\cS \times   \cS} \mut(s,s')  \log  \int_{\cA} \pi(a|s) \cP(s'|s,a) da ds' ds \\
%     &\lkxcom{=} H(\mut(s'|s))   +  \int_{\cS \times   \cS} \mut(s,s')   \int_{\cA}  \underbrace{   \PI^*(a|s,s') \cP(s'|s,a) }_{\text{ \eq{ \ref{eq:inverse} }}}   da ds' ds. \\
% \end{align*} 

% \vskip -0.1 in
% $\cD_\KL[\mut(s'|s) || \mupi(s'|s)] $ is minimized when $\pi$ follows $\PI^*(\cdot|s,s')$: $$\pi(\cdot|s) \propto \PI^*(\cdot|s,s') ~ \forall s, s \sim \mut(s,s').$$ 
% \end{proof}
% Intuitively, this constraint encourages \textit{mode-covering}, by leading policy to take actions that \textit{cover} the ideal next state. Since $\PI^*(\cdot|s,s')$ only has \textit{support} on actions that yields transition $s \to s'$, following this constraint can avoid policy from deviating to other states. 

{\lemma \label{lemma:bc-lowerbound-reverse}:
    \begin{align*}
        \cD_\KL[\pi(a|s)||\pi_E(a|s)] = \cD_\KL[\mupi(s'|s)||\mut(s'|s)] +  \cD_\KL[\mupi(a|s,s')||\mut(a|s,s')].  
    \end{align*}
}  
\begin{proof}
    Based on the definition of $\mupi(a|s,s')$: 
    \begin{align} \label{eq:invese-def}
        \mupi(a|s,s')= \frac{\pi(a|s) \cP(s'|s,a)}{\int_\cA \pi(\ba|s) \cP(s'|s,\ba)d\ba} = \frac{\pi(a|s) \cP(s'|s,a)}{\mupi(s'|s)},    
    \end{align}
    and similar for $\mut(a|s,s')$, we can derive:
    \begin{align*}
        &\cD_\KL[\pi(a|s) || \pi_E(a|s)] \\
        = & \int_{\cS \times \cA} \mupi(s,a)  \log \frac{\pi(a|s)} {\pi_E(a|s)} da ds \\
        = & \int_{\cS \times \cA \times \cS} \mupi(s,a)  \log \frac{\pi(a|s)} {\pi_E(a|s)} ds' da ds\\
        = & \int_{\cS \times \cA \times \cS} \mupi(s,a,s') \log \frac{\pi(a|s) \cP(s'|s,a)  } {\pi_E(a|s) \cP(s'|s,a) } ds'da ds \\
        = & \int_{\cS \times \cA \times \cS} \mupi(s,a,s') \underbrace{\log \frac {\mupi(a|s,s') \mupi(s'|s) }{ \mut(a|s,s') \mut(s'|s) }} _{\text{ \eq{\ref{eq:invese-def}}}} ds'da ds \\
        = & \int_{\cS \times \cA \times \cS} \mupi(s,a,s') \Big( \log \frac{ \mupi(a|s,s')  } {\mut(a|s,s') } + \log \frac{\mupi(s'|s)}{\mut(s'|s)} \Big) ds' da ds \\
        = & \int_{\cS \times \cA \times \cS} \mupi(s,a,s')  \log \frac{ \mupi(a|s,s')  } {\mut(a|s,s') } ds' da ds + \int_{\cS \times \cA \times \cS} \mupi(s,a,s') \log \frac{ \mupi(s'|s)  } {\mut(s'|s) } ds' da ds \\
        = & \cD_\KL[\mupi(a|s,s') || \mut(a|s,s')] +  \cD_\KL[\mupi(s'|s)||\mut(s'|s)].
    \end{align*}
\end{proof}

\textbf{Lemma \ref{lemma:bc-lowerbound}:}  
    \begin{align*}
        \cD_\KL[\pi_E(a|s)||\pi(a|s)] = \cD_\KL[\mut(s'|s)||\mupi(s'|s)] +  \cD_\KL[\mut(a|s,s')||\mupi(a|s,s')].  
    \end{align*}
Proof is same as Lemma \ref{lemma:bc-lowerbound-reverse} by switching $\pi$ with $\pi_E$.
% \begin{proof}
%     Based on the definition of $\mupi(a|s,s')$: 
%     \begin{align} \label{eq:invese-def}
%         \mupi(a|s,s')= \frac{\pi(a|s) \cP(s'|s,a)}{\int_\cA \pi(\ba|s) \cP(s'|s,\ba)d\ba} = \frac{\pi(a|s) \cP(s'|s,a)}{\mupi(s'|s)},    
%     \end{align}
%     and similar for $\mut(a|s,s')$, we can derive:
%     \begin{align*}
%         &\cD_\KL[\pi_E(a|s) || \pi(a|s)] \\
%         = & \int_{\cS \times \cA} \mut(s,a)  \log \frac{\pi_E(a|s)} {\pi(a|s)} da ds \\
%         = & \int_{\cS \times \cA \times \cS} \mut(s,a)  \log \frac{\pi_E(a|s)} {\pi(a|s)} ds' da ds\\
%         = & \int_{\cS \times \cA \times \cS} \mut(s,a,s') \log \frac{\pi_E(a|s) \cP(s'|s,a)  } {\pi(a|s) \cP(s'|s,a) } ds'da ds \\
%         = & \int_{\cS \times \cA \times \cS} \mut(s,a,s') \underbrace{\log \frac{ \mut(a|s,s') \mut(s'|s) } {\mupi(a|s,s') \mupi(s'|s) }}_{\text{ \eq{\ref{eq:invese-def}}}} ds'da ds \\
%         = & \int_{\cS \times \cA \times \cS} \mut(s,a,s') \Big( \log \frac{ \mut(a|s,s')  } {\mupi(a|s,s') } + \log \frac{\mut(s'|s)}{\mupi(s'|s)} \Big) ds' da ds \\
%         = & \int_{\cS \times \cA \times \cS} \mut(s,a,s')  \log \frac{ \mut(a|s,s')  } {\mupi(a|s,s') } ds' da ds + \int_{\cS \times \cA \times \cS} \mut(s,a,s') \log \frac{ \mut(s'|s)  } {\mupi(s'|s) } ds' da ds \\
%         = & \cD_\KL[\mut(a|s,s') || \mupi(a|s,s')] +  \cD_\KL[\mut(s'|s)||\mupi(s'|s)].
%     \end{align*}

% \end{proof}
%while the main objective works by encouraging \textit{mode seeking}.

%Operator $\cB^\pi$ depends on a synthetic reward from discriminator, optimized by \eq{\ref{eq:offpolicy-d}}. 
\subsection{ Derivation of \eq{\ref{obj:main-dice}}:} \label{Appendix:obj:main-dice}
\begin{align*} %\label{obj:main-dice-prove}
    %\JOPOLO(\pi, Q) &=  \cE_{(s, a, s')\sim \mupi(s, a, s')}[ r(s,s') - (\cB^\pi Q - Q)(s,a)] + \alpha E_{(s,a) \sim \muR}[f_*(\frac{1}{\alpha}(\cB^\pi Q - Q)(s,a))]  
    \JOPOLO(\pi, Q) &=  \cE_{(s, a, s')\sim \mupi(s, a, s')}[ r(s,s') - (\cB^\pi Q - Q)(s,a)] +  E_{(s,a) \sim \muR}[f_*((\cB^\pi Q - Q)(s,a))],  
\end{align*}
where $\cB^\pi Q(s,a)= \cE_{s'\sim P(\cdot|s,a),a' \sim \pi(\cdot|s')}\Big [r(s,s') + \gamma Q(s',a') \Big].$ 
\begin{proof}
    The first term in the RHS can be reduced to the following:
\begin{align*} 
   &\cE_{(s, a, s')\sim \mupi(s, a, s')}[ r(s,s') - (\cB^\pi Q - Q)(s,a)]  \\
   = &\cE_{(s, a)\sim \mupi(s, a)}\Big[ \cE_{s' \sim \cP(\cdot|s,a)} [r(s,s') ]- \cE_{s' \sim \cP(\cdot|s,a)} [(\cB^\pi Q - Q)(s,a)] \Big]  \\
   = &\cE_{(s, a)\sim \mupi(s, a)}\Big[ \cE_{s' \sim \cP(\cdot|s,a)} [r(s,s') ] + Q(s,a) - \cE_{s' \sim \cP(\cdot|s,a)} [\cB^\pi Q (s,a)] \Big]  \\
   = &\cE_{(s, a)\sim \mupi(s, a)}\Big[ \cE_{s' \sim \cP(\cdot|s,a)} [r(s,s') ] + Q(s,a) - \cE_{s' \sim \cP(\cdot|s,a), a' \sim \pi(\cdot|s')} [ r(s,s') + \gamma  Q (s',a')] \Big]  \\
   = &\cE_{(s, a)\sim \mupi(s, a)}[Q(s,a)- \gamma \cE_{s' \sim \cP(\cdot|s,a), a' \sim \pi(\cdot|s')} [Q(s',a' )] ] \\
   = & (1-\gamma)\sum_{t=0}^{\infty} \gamma^t \cE_{s \sim \mu^\pi_t, a \sim \pi(s)}[Q(s,a)] - (1-\gamma)\sum_{t=0}^{\infty} \gamma^{t+1} \cE_{s \sim \mu^\pi_t, a \sim \pi(\cdot|s),s' \sim \cP(\cdot|s,a), a' \sim \pi(\cdot|s')} [Q(s',a' )] ]  \\
   = & (1-\gamma)\sum_{t=0}^{\infty} \gamma^t \cE_{s \sim \mu^\pi_t, a \sim \pi(s)}[Q(s,a)] - (1-\gamma)\sum_{t=0}^{\infty} \gamma^{t+1} \cE_{s \sim \mu^\pi_{t+1}, a \sim \pi(\cdot|s) } [Q(s,a)] ]  \\
   = & (1-\gamma) \cE_{s\sim p_0, a_0 \sim \pi(\cdot|s_0)}[Q(s_0,a_0)]
\end{align*}
Therefore:
%$$\JOPOLO(\pi, Q) = (1-\gamma) \cE_{s\sim p_0, a_0 \sim \pi(s_0)}[Q(s_0,a_0)] + \alpha E_{(s,a) \sim \muR}[f_*(\frac{1}{\alpha}(\cB^\pi Q - Q)(s,a))].$$ 
$$\JOPOLO(\pi, Q) = (1-\gamma) \cE_{s\sim p_0, a_0 \sim \pi(\cdot|s_0)}[Q(s_0,a_0)] +  E_{(s,a) \sim \muR}[f_*((\cB^\pi Q - Q)(s,a))].$$ 
\end{proof}
